# Supplementary material for: Unity in Diversity: Multi-expert Knowledge Confrontation and Collaboration for Generalizable Vehicle Re-identification
Source: arXiv:2407.07351 source file (2025-02-04)
Supplement: Supplementary file 1 [file X_suppl.tex]

\clearpage
\setcounter{page}{1}
\maketitlesupplementary

\section{The Loss Functions of CLIP-ReID}
\label{sec:c1}
CLIP-ReID\cite{r18} proposes a dual-stage training strategy to learn the identity-specific text prompts and finetune the global visual features with the supervision of learned text prompts. In our proposed work, CLIP-ReID is set as the baseline model. The loss function of MiKeCoCo in the first stage follows the design of CLIP-ReID which utilizes the CLIP-style contrastive losses $\mathcal{L}_{v2t}$ and $\mathcal{L}_{t2v}$. The formula in MikeCoCo is as below:
\begin{equation}\label{formula16}
	\begin{aligned}
		\mathcal{L}_{v2t} = \sum_{k=1}^{K}\frac{-1}{|P(y_{n})|}\sum_{p \in P(y_{n})}log\frac{exp\big(s(f_{n}^{k}, T_{y_{n}}^k)\big)}{\sum_{y_{a}=1}^{N}exp\big(s(f_{n}^{k}, T_{y_{a}}^k)\big)},
	\end{aligned}
\end{equation}
\begin{equation}\label{formula17}
	\begin{aligned}
		\mathcal{L}_{t2v} = \sum_{k=1}^{K}\frac{-1}{|P(y_{n})|}\sum_{p \in P(y_{n})}log\frac{exp\big(s(f_{n}^{k}, T_{y_{n}}^k)\big)}{\sum_{a=1}^{N}exp\big(s(f_{a}^{k}, T_{y_{n}}^k)\big)},
	\end{aligned}
\end{equation}
where $s(\bigcdot)$ denotes the similarity calculation, $|\bigcdot|$ is the cardinality of predictions and $T_{y_{n}}^k$ denotes the learned text embeddings of $n$-th ID from the $k$-th expert.

In the second training stage, visual-text matching loss $\mathcal{L}_{v2tce}$ is employed to utilize the learned text prompts as the ID Classifier. The optimization of the loss in MikeCoCo is calculated as below:
\begin{equation}\label{formula20}
	\begin{aligned}
		\mathcal{L}_{v2tce}= -\frac{1}{K}\sum_{k=1}^{K}\sum_{n=1}^{N}q_{n}^klog\frac{exp\big(s(f_{n}^k, T_{y_{n}}^k)\big)}{\sum_{y_{n}^a=1}^{N}exp\big(s(f_{n}^k, T_{y_{a}}^k)\big)}.
	\end{aligned}
\end{equation}

\begin{table*}[ht!]
 \caption{
    Domain generalization performance comparison with person datasets as the target domain. The cumulative matching rate(\%) and mean Average Precision (mAP)(\%) are listed. `--' denotes that no reported result is available. The best and second best results are marked in \textbf{bold} and \underline{underline}, respectively.
    }
    %\scriptsize  %字体大小
    \centering
    \resizebox{\linewidth}{!}
    {
    \begin{tabular}{c|c|cc|cc|cc}\hline 
        \multirow{2}{*}{\textbf{Methods}} & \multirow{2}{*}{\textbf{Venue}} &  \multicolumn{2}{c|}{\textbf{Market$\to$MSMT17}} & \multicolumn{2}{c|}{\textbf{Market$\to$CUHK-NP}} & \multicolumn{2}{c}{\textbf{MSMT17$\to$CUHK-NP}}\\ \cline{3-8}
      & & Rank-1  & mAP  & Rank-1  & mAP & Rank-1  & mAP \\ \hline
      CNB              & ECCV'20  & 25.3    & 9.2     & --     &   --     &   --   & --   \\
      OSNet        & TPAMI'21 & 23.5    & 8.2     & --     &   --     &   --   & --   \\  \hline
      QAConV           & ECCV'20  & 22.6    & 7.0     & 9.9    &   8.6    & \textbf{25.3}   & 22.6 \\
      TransMatcher-GS   & NIPS'21  & 47.3    & 18.4    & 22.2   &   21.4   & 23.7   & 22.5 \\
      QAConv-GS         & CVPR'22  & 45.9    & 17.2    & 19.1   &   18.1   & 20.9   & 20.6 \\
      MAD                        & CVPR'22  & 33.5    & 11.8    & --     &   --     &   --   & -- \\
      MSI-Net        & CVPR'23  & 22.4    & 8.3     & --     &   --     &   --   & -- \\
      PAT             & ICCV'23  & 42.8    & 18.2    & \textbf{25.4}   &   \textbf{26.0}   &  \underline{24.2}    & \textbf{25.1} \\
      MiKeCoCo!                  & This Venue  &  \textbf{49.0}   & \underline{18.8}        &   23.3  & 22.7       & 21.0     & 19.9 \\
      MiKeCoCo                   & This Venue &  \underline{48.6}   & \textbf{19.4}        &   \underline{24.4}  & \underline{24.1}       & 24.1     & \underline{23.8} \\
        \hline 
    \end{tabular}
}
    \label{pr}
\end{table*}

\section{The Design of Band-pass Filter for STREAM}

In the strategy of STREAM, a band-pass filter $\mathcal{M}(r)$ is designed as a mask to split non-causal parts (extremely high and low frequency) and causal parts (other frequency) of the source images $X_{s}$ in the frequency spectrum. The frequency spectrum $DCT(X_{s})$ are firstly obtained and then decomposed into four frequency parts through the cut-off frequency point sets $v=\left \{ v_{1}, v_{2}, v_{3} \right \}$. The formulations are as follows:

\begin{equation}\label{formula7}
	\begin{aligned}
	\mathcal{M}(r)=\left\{\begin{matrix}
     \mathcal{M}_{1}(r), & r\le v_{1},  \\
     \mathcal{M}_{2}(r), & v_{1} < r\le v_{2},  \\
     \mathcal{M}_{3}(r), & v_{2} < r\le v_{3},  \\
     \mathcal{M}_{4}(r), & r>v_{3}.
    \end{matrix}\right.
	\end{aligned}
\end{equation}
For $m_{1}(i, j)$ of the low frequency part $\mathcal{M}_{1}(r)$ in the $(i, j)$ position is defined as below:
\begin{equation}\label{formula7}
	\begin{aligned}
	    m_{1}(i,j) = 1-\frac{c_{1}}{v_{1}}max(i,j),
	\end{aligned}
\end{equation}
where $c_{1}$ is the coefficient of $m_{1}(i,j)$, we set it as 0.95. And $m_{3}(i, j)$ of the high frequency part $\mathcal{M}_{3}(r)$ in the $(i, j)$ position is defined as below:
\begin{equation}\label{formula7}
	\begin{aligned}
	    m_{3}(i,j) = \frac{c_{2}}{v_{3}-v_{2}}max(i,j).
	\end{aligned}
\end{equation}
where $c_{2}$ represents the coefficient of $m_{1}(i,j)$, the value of it is 0.3. The band-pass frequency part and the extremely high frequency part are denoted as $\mathcal{M}_{2}(r)$ and $\mathcal{M}_{4}(r)$, they are set to the constant values 0.01 and 0.5, respectively.

Besides, the cut-off frequency point sets $v$ are calculated as below:
\begin{equation}\label{formula7}
	\begin{aligned}
	    v_{i} = min(H, W)\cdot k_{i}, \quad with~i=1,2,3,
	\end{aligned}
\end{equation}
where H and W represent the height and width of the frequency spectrum. The hyper-parameters $k_{1}$, $k_{2}$ and $k_{3}$ are 0.005, 0.7 and 1.0, respectively.

\begin{figure}[h!]
    \centering
    \includegraphics[width=3.25in,height=2.85in]{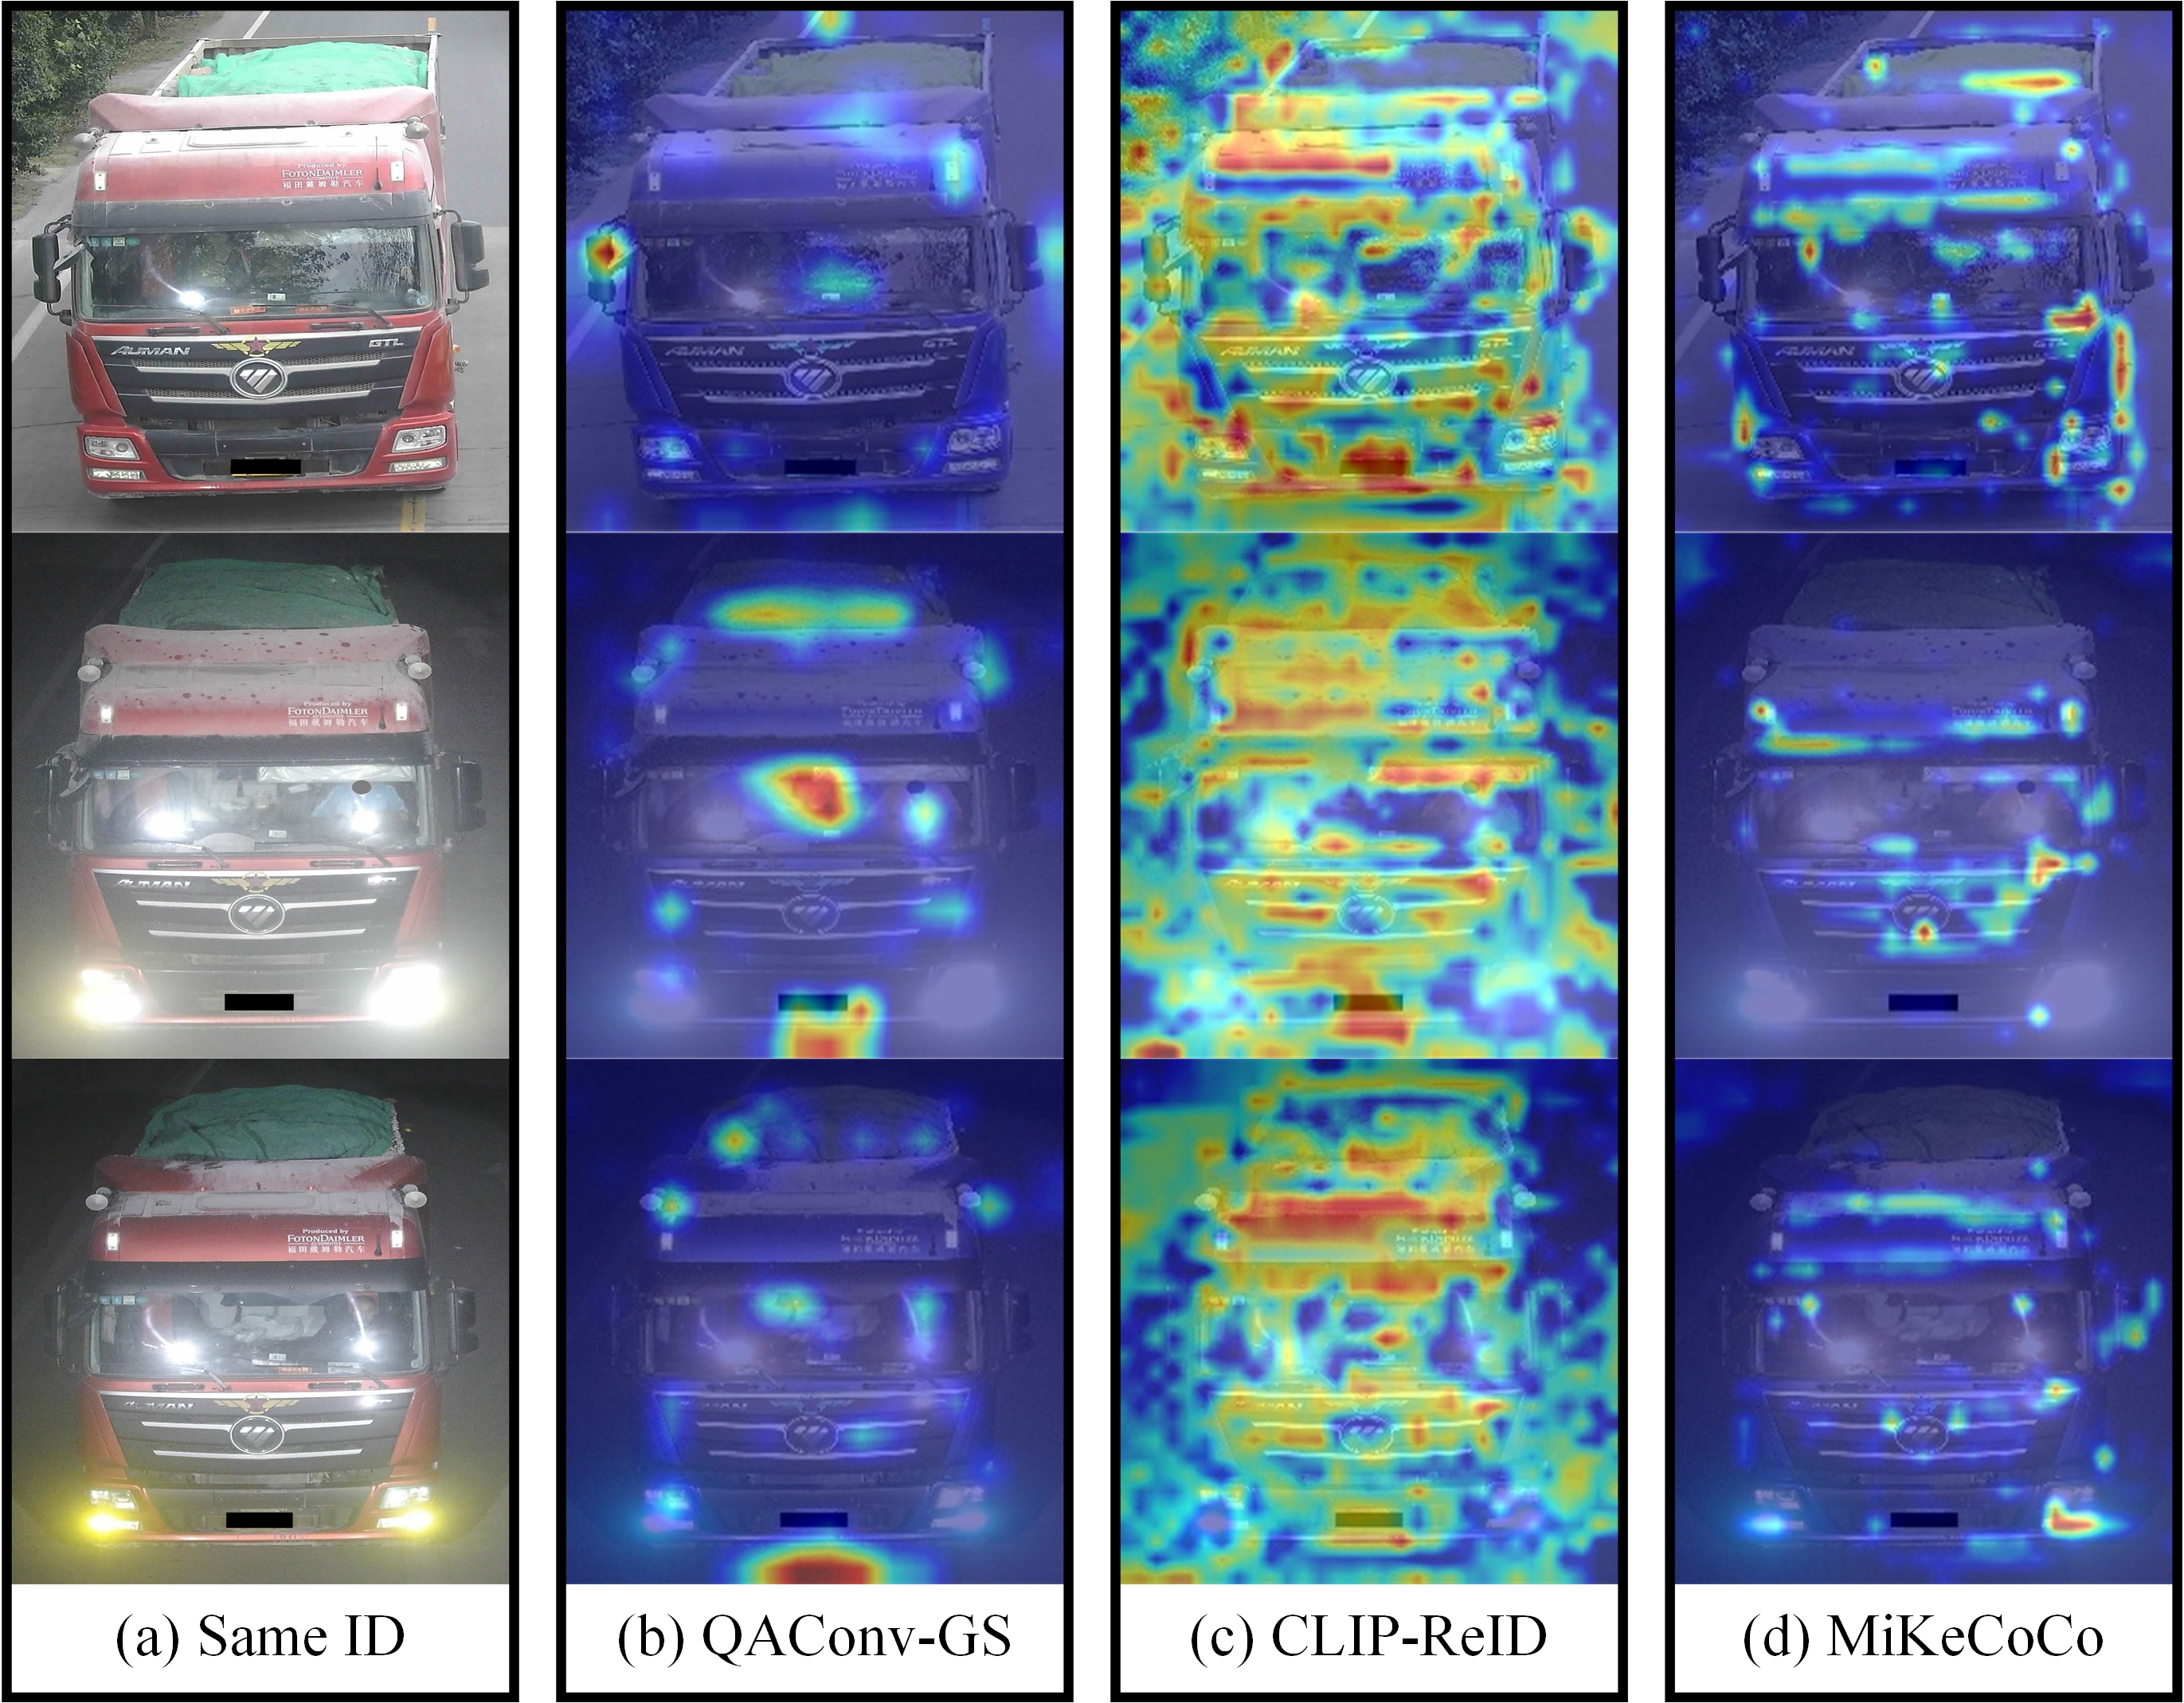}
	\caption{Visualization of activation maps of three different methods on the VeRi--776$\to$Opri setting.}
	\label{gradcam}
\end{figure}

\begin{figure}[ht!]
	\centering
\includegraphics[width=3.3in,height=4.6in]{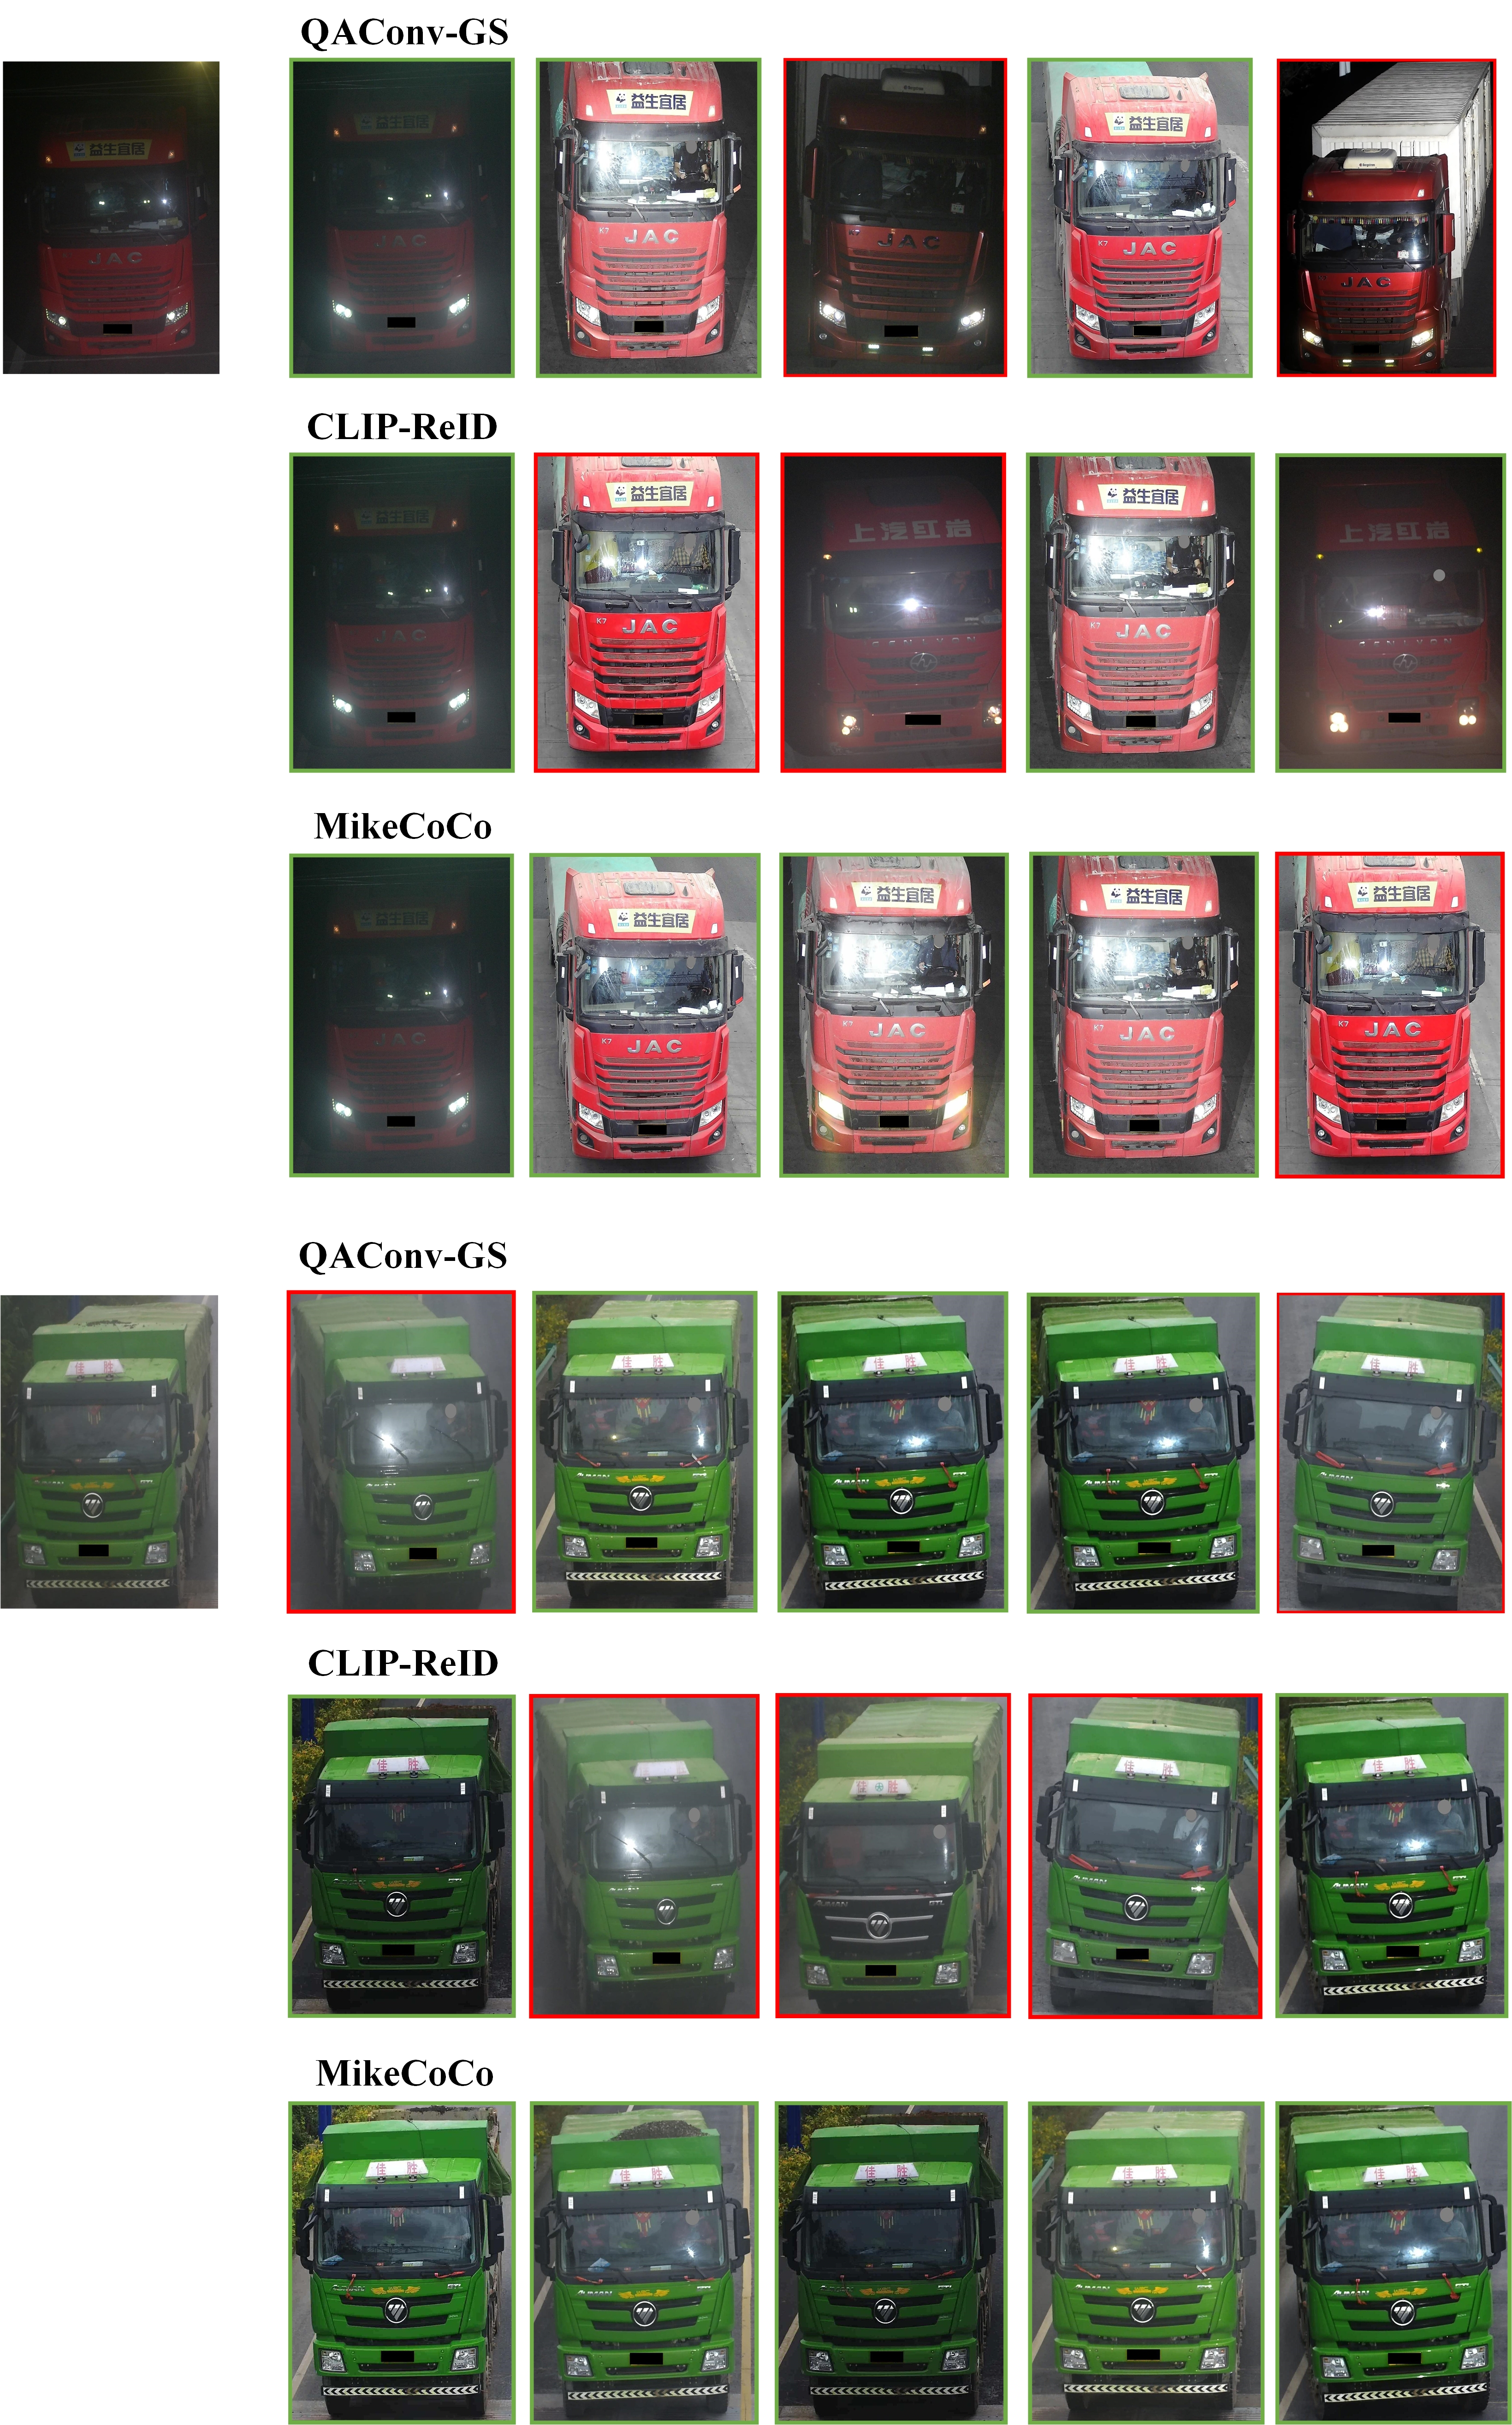}
	\caption{The examples of the top-5 retrieval results on Opri dataset. The retrieval results showcase the identification performance of the QAConv-GS, CLIP-ReID, and MikeCoCo methods on the VeRi--776$\to$Opri setting. The \textbf{green} and \textbf{red} boxes indicate correct and error retrieval results respectively.}
	\label{retrieval}
\end{figure}

\section{Visualization}
\subsection{Visualization of Feature Maps}
To explore the focused areas of the our proposed model, visualization experiments using grad-CAM~\cite{s4} are conducted to obtain the activation maps of QAConv-GS, CLIP-ReID and MikeCoCo in Fig.\ref{gradcam}. We can observe that MiKeCoCo pays more attention to identity-related discriminate features, while QAConv-GS focuses on the unrelated local areas (e.g., drivers and vehicle licenses). The attention of the feature maps in the CLIP-ReID method is scattered. In contrast, MiKeCoCo proposed in this paper can focus on the same feature region of different samples with the same vehicle. Thus our method can extract identity-related features effectively.

\subsection{Visualization of Retrieval Result}
We visualize the top-5 retrieval results of three methods (QAConv-GS, CLIP-ReID and MikeCoCo) on Opri in Fig.\ref{retrieval}, with the incorrectly identified samples highlighted in red and the correct samples are marked in green.

\section{Comparison with State-of-the-art Methods on Person ReID Datasets}
To further validate the generalization capability of the proposed model, we conduct experiments using the commonly used person re-identification datasets: Market-1501~\cite{d2}, MSMT17~\cite{d3}, and CUHK03~\cite{d4}. In these experiments, Market-1501 and MSMT17 serve as the source domains, with MSMT17 also serving as the target domain. Furthermore, the challenging protocols of CUHK03-NP~\cite{d1} are adopted as the target domain. The training parts of Market-1501 dataset contain 12,936 images from 751 identities, and the test subset is composed of 19,732 images with 750 persons. The MSMT17 dataset includes 126,411 images with 4,101 identities. It is split into a training set of 32,621 images from 1,041 identities, the remaining test set contains 93,820 images with 3,010 persons. The CUHK03-NP includes 767 and 700 persons used for training and testing, respectively.

Table \ref{pr} provides a comparison of experimental results for state-of-the-art domain generalization methods in person ReID. The recently published methods are compared following the evaluation protocol for domain generalization ReID, including CNB~\cite{s3}, OSNet-AIN~\cite{r64}, QAConV~\cite{s2}, TransMatcher-GS~\cite{r7}, QAConv-GS~\cite{r8}, MAD~\cite{r14}, MSI-Net~\cite{r65} and PAT~\cite{r70}. Note that, TransMatcher-GS denotes that graph sampling strategy~\cite{r8} is utilized in TransMatcher model. Besides, MikeCoCo outperforms the SOTA method by 1.7$\%$ and 1.0$\%$ on mAP and Rank-1 in Market $\to$ MSMT17 scenario, which demonstrates the effectiveness and superiority of our method. MikeCoCo with three experts also achieves competitive performance compared to other methods in the MSMT17 $\to$ CUHK-NP scenario. Experimental results demonstrate that MiKeCoCo not only performs exceptionally well in domain generalization for vehicle re-identification but also shows potential for extending to person ReID tasks.
