# Supplementary material for: Unity in Diversity: Multi-expert Knowledge Confrontation and Collaboration for Generalizable Vehicle Re-identification
Source: arXiv:2407.07351 source file (2025-02-04)
Supplement: Supplementary file 2 [file supplementary.tex]

\section{Appendix Section}
\label{sec:appendix_section}
Supplementary material goes here.
